# Supplementary material for: StyleDrop: Text-to-Image Generation in Any Style
Source: arXiv:2306.00983 source file (2023-06-01)
Supplement: Supplementary file 1 [file supp_ablation_multi_concept.tex]

\begin{figure}
    \centering
    \includegraphics[width=0.99\linewidth]{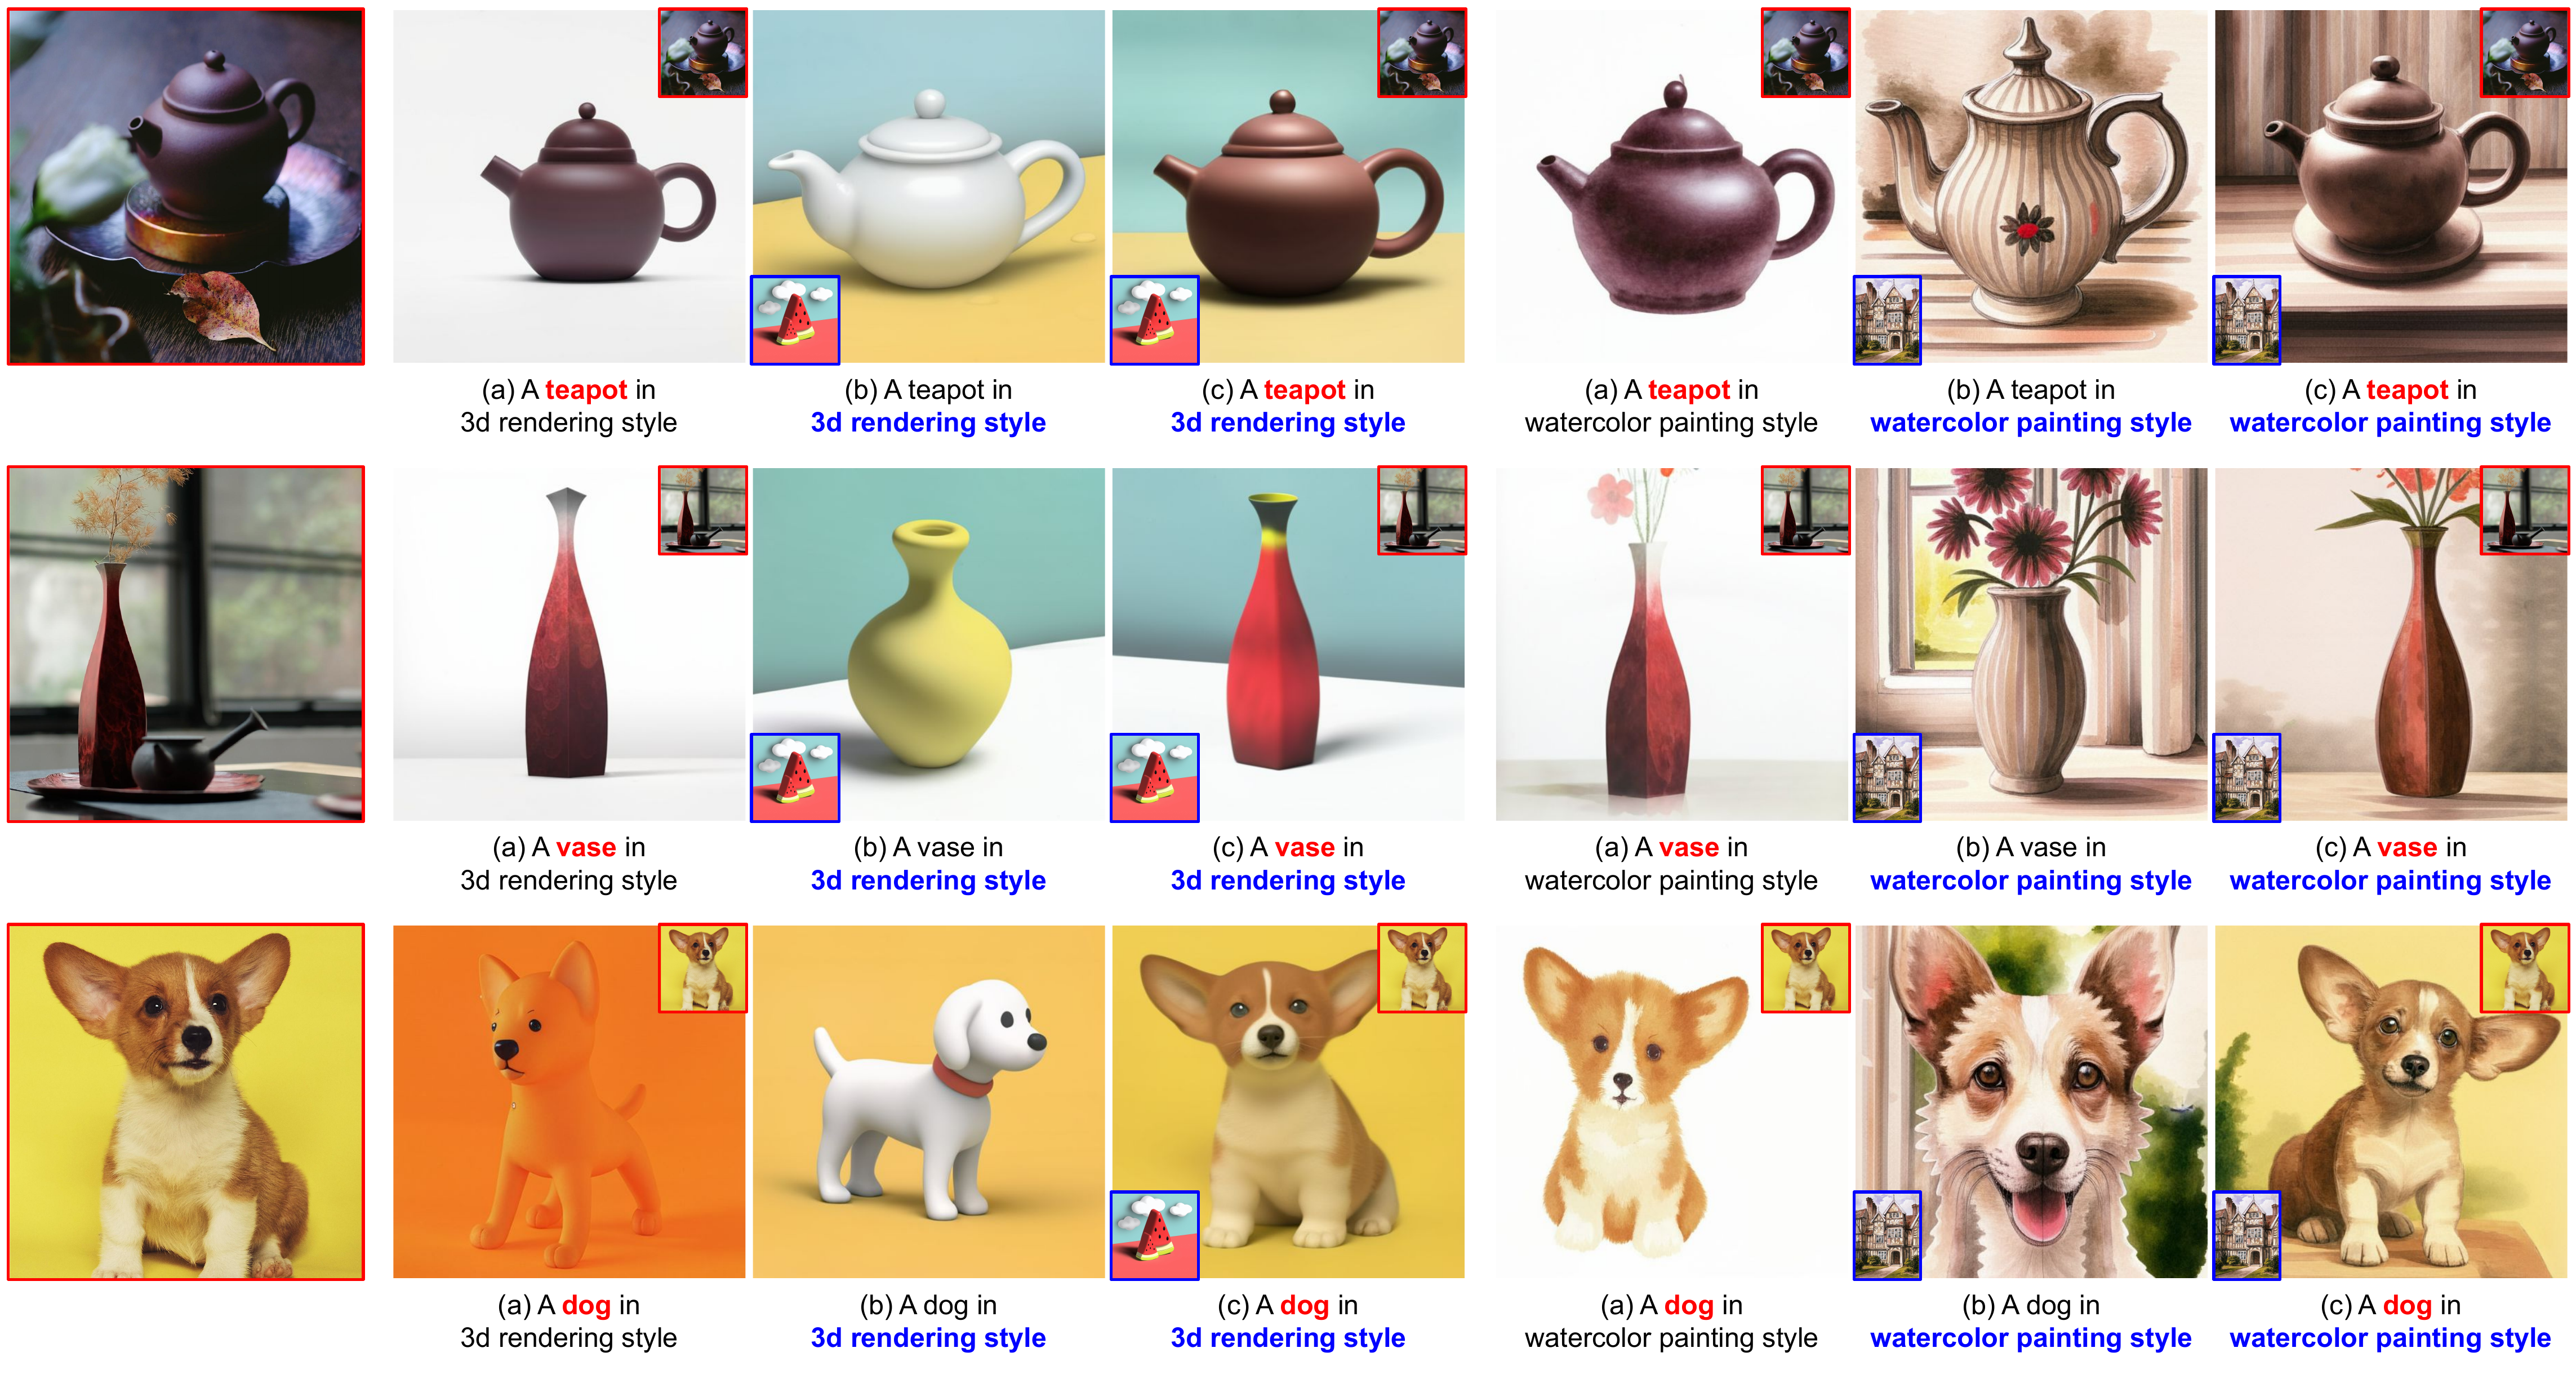}
    \caption{{\color{red}[[PLACEHOLDER for MULTI-CONCEPT JOINT TRAINING ABLATION]]}}
    \label{fig:supp_ablation_multi_concept}
\end{figure}
